# Supplementary material for: Low-Regret Active learning
Source: arXiv:2104.02822 source file (2022-02-22)
Supplement: Supplementary file 1 [file appendix.tex]

\input{supp/results.tex}

% \section{Additional Evaluations}
% \label{sec:supp-add-eval}

% \section{Additional Evaluations}
% \label{sec:supp-eval-adaprod}
